# Supplementary material for: Dynamic Control of Nonequilibrium Metal-Insulator Transitions
Source: arXiv:2004.04669 source file (2020-04-09)
Supplement: Supplementary file 1 [file suppinfo.pdf]

# Dynamic Control of Nonequilibrium Metal–Insulator Transitions: Supporting Information

Joseph Kleinhenz,† Igor Krivenko,† Guy Cohen,*,‡ and Emanuel Gull*,†

†*Department of Physics, University of Michigan, Ann Arbor, Michigan 48109, USA*

‡*School of Chemistry, Tel Aviv University, Tel Aviv 69978, Israel*

E-mail: gcohen@tau.ac.il; egull@umich.edu

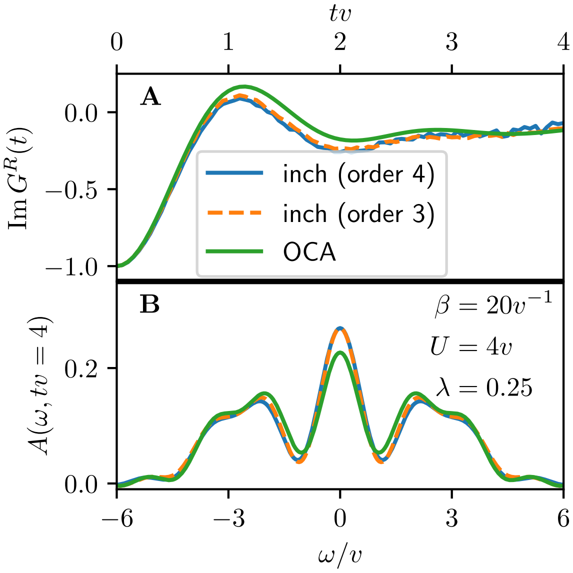


Figure S1: Comparison of the retarded Green's function (**A**) and spectral function (**B**) obtained from OCA (green) and inchworm (blue/orange) at $\beta = 20v^{-1}$, $U = 4.0v$, $\lambda = 0.25$.

Fig. S1 shows a comparison between results obtained using the one crossing approximation (OCA) and the inchworm QMC method. The parameters are chosen in order to

make the inchworm calculations computationally feasible. The inchworm results are fully converged with order and numerically exact. The OCA somewhat underestimates the height of the quasi-particle peak but otherwise captures the spectrum well. These results support the reliability of OCA in capturing the real-time dynamics of the system.
